# Supplementary material for: EmbedJoin: Efficient Edit Similarity Joins via Embeddings
Source: arXiv:1702.00093 source file (2017-10-06)
Supplement: Supplementary file 1 [file appendix.tex]

\section{A Running Example for EmbedJoin}
\label{sec:example}

\begin{table}[h]
\begin{minipage}[]{0.25\textwidth}
\centering
\begin{tabular}{ |l|l| }
  \hline
  \multicolumn{2}{|c|}{Strings} \\
  \hline
  $s_1$ & ACGTGACGTG \\
  $s_2$ & ACGTCGCGTG\\
  $s_3$ & ACTTACCTG \\
  $s_4$ & ATCGATCGGT\\
  \hline
\end{tabular}
\centerline{(a)}
\end{minipage}
\begin{minipage}[]{0.2\textwidth}
\centering
\begin{tabular}{ |l|l| }
  \hline
  \multicolumn{2}{|c|}{LSH functions } \\
  \hline
  $f_1^1$ & ($h_2$,$h_9$) \\   \hline
  $f_2^1$ &  ($h_1$,$h_4$) \\   \hline
  $f_1^2$ &  ($h_2$,$h_5$)  \\   \hline
  $f_2^2$ &  ($h_7$,$h_3$) \\
  \hline
\end{tabular}
\centerline{(b)}
\end{minipage}
\caption{A collection of strings and LSH functions}  
\label{tab:strs}
\end{table}

\begin{table}[]
\begin{minipage}[]{0.49\textwidth}
\centering
\begin{tabular}{l*{10}{c}r}
\ $j$              & 1 & 2 & 3 & 4 & 5  & 6 & 7 & 8  & 9 & 10 & $\dots$  \\
\hline
$\pi_j(A)$    & 0 & 1 & 0 & 0 & 1 & 0 & 1 & 1 & 0 & 1  & $\dots$\\
$\pi_j(C)$     & 1 & 1 & 0 & 1 & 1 & 1 & 1 & 0 & 0 & 0 & $\dots$ \\
$\pi_j(G)$    & 0 & 1 & 1 & 1 & 0& 0 & 0 & 1 & 1 & 1  & $\dots$\\
$\pi_j(T)$     & 1 & 0 & 0 & 0 & 1 & 0 & 1 & 1 & 0 & 1  & $\dots$ \\
\end{tabular}
\centerline{(a) Random string $R^1$}
\end{minipage}
\begin{minipage}[]{0.49\textwidth}
\centering
\begin{tabular}{l*{10}{c}r}
\ $j$              & 1 & 2 & 3 & 4 & 5  & 6 & 7 & 8  & 9 & 10 & $\dots$  \\
\hline
$\pi_j(A)$    & 1 & 0 & 0 & 0 & 1 & 0 & 0 & 0 & 1 & 0  & $\dots$\\
$\pi_j(C)$     & 1 & 1 & 0 & 0 & 1 & 1 & 1 & 1 & 0 & 0 & $\dots$ \\
$\pi_j(G)$    & 1 & 0 & 1 & 1 & 0& 0 & 1 & 1 & 0 & 1  & $\dots$\\
$\pi_j(T)$     & 1 & 0 & 0 & 1 & 0 & 1 & 1 & 1 & 0 & 0  & $\dots$ \\
\end{tabular}
\centerline{(b) Random string $R^2$}
\end{minipage}
 \caption{Random strings for two CGK embeddings; represented as the equivalent $\pi_j(\cdot)$'s} 
\label{tab:CGK}
\end{table}

\begin{table}[]
\centering
\begin{tabular}{ |l|l| } 
  \hline
  \multicolumn{2}{|c|}{Strings after embedding} \\
  \hline
  $t_1^1$ & AACCGGGGTT $\dots$ \\
  $t_1^2$ & ACGTGGGAAC $\dots$\\
  $t_2^1$ & AACCGGGGTT $\dots$\\
  $t_2^2$ & ACGTCGGCGG $\dots$\\
  $t_3^1$ & AACCTTTACC $\dots$\\
  $t_3^2$ & ACTTTTAAAC $\dots$\\
  $t_4^1$ & AATTTCGGAA $\dots$\\
  $t_4^2$ & ATTTCGGAAT $\dots$\\
  \hline
\end{tabular}
\caption{Strings after embedding}  
\label{tab:strs2}
\end{table}

\begin{table}[!]
\centering
\begin{tabular}{l*{3}{c}r}
\ $i$              &$f_1^1(t_i^1)$  &$f_2^1(t_i^1)$ & $f_1^2(t_i^2)$ & $f_2^2(t_i^2)$   \\
\hline
$1$    & (A,T) & (A,C) & (C,G) & (G,G) \\
$2$     & (A,T) & (A,C) & (C,C) & (G,G)  \\
$3$    & (A,C) & (A,C) & (C,T) & (A,T) \\
$4$     & (A,A) & (A,T) & (T,C) & (G,T)  \\
\end{tabular}
\caption{Signatures of LSH functions}  
\label{tab:lshvalue}
\end{table}

Table~\ref{tab:strs}(a) shows the collection of input strings, and the set of LSH functions we use. Set distance threshold $K=3$. We choose parameters $r=2, z=2, m=2$ for \ebdjoin.  
Table~\ref{tab:CGK} shows two random strings $R^1, R^2$ (represented as the equivalent $\pi_j(\cdot)$'s; see Algorithm~\ref{alg:CGK}) that we use for the two rounds of CGK-embeddings. Table~\ref{tab:strs2} shows the strings after CGK-embedding, and Table~\ref{tab:lshvalue} shows the signatures of LSH functions. From Table~\ref{tab:lshvalue} we find that $f_1^1(t_1^1)=f_1^1(t_2^1)=(A,T)$, $f_2^1(t_1^1)=f_2^1(t_2^1)=f_2^1(t_3^1)=(A,C), f_2^2(t_1^2)=f_2^2(t_2^2)=(G,G)$, and thus $ (s_1,s_2),(s_1,s_3),(s_2,s_3)$ are candidate pairs.  Finally after the verification step, we output $(s_1,s_2)$, $(s_1,s_3)$ as the results of similarity joins.
